# Supplementary material for: All that is English may be Hindi: Enhancing language identification through automatic ranking of likeliness of word borrowing in social media
Source: arXiv:1707.08446 source file (2017-07-29)
Supplement: Supplementary file 1 [file 70Appendix.tex]

\begin{appendix}
\section{Examples of English-Hindi bilingual tweets}
Figure~\ref{fig:ex} presents examples of some typical English-Hindi bilingual tweets occurring in SMC.

\begin{figure}
\caption{Some example code-mixed tweets from English-Hindi bilinguals. Hindi words are in italics.}
\fbox{\begin{centering}\begin{minipage}{0.4\textwidth}
{\tt Huge traffic restrictions for PM's visit to \#blast site mean deserted roads in \#Hyderabad. \textit{``Itna sanaata kyon hai bhai?''}}\\
{\bf Translation}: Huge traffic restrictions for Prime Minister's visit to the blast site mean deserted roads in Hyderabad. ``Why is there so much silence, bro?''\\
\\
{\tt MMS  will go to \#HyderabadBlast site to take \textit{jayeja} of area \& say \textit{Hazaaron Jawabon Se Acchi Hai Meri Khamoshi} \#ThikHai}\\
{\bf Translation}: MMS (name of a politician) will go to \#HyderabadBlast site to take a survey of the area and say "My silence is better than a thousand answers." \#ThikHai
\end{minipage}
\end{centering}
}
\label{fig:ex}
\end{figure}

\section{Tweet type distribution in dataset}
The details of the number and \% of tweets falling in each of the six tweet categories introduced in section~4 of the main text are presented in table~\ref{tab:stat}.

\begin{table}
%\vspace{-2mm}
\centering
\scalebox{0.8}{
\begin{tabular}{|l|l|l|l|}
\hline 
Type & Number of Tweets & percentage \\ \hline \hline
\textit{En}  & 645655 & 81.97 \\ \hline
\textit{Hi}   & 24960 &  3.16 \\ \hline
\textit{CME}  & 31998  & 4.06 \\ \hline
\textit{CMH}  & 39877 & 5.06 \\ \hline
\textit{CMEQ} & 3584    & 0.455 \\ \hline
\textit{CS} & 41532  & 5.27 \\ \hline
\end{tabular}
}
%\vspace{-4mm}
\caption{Number and percentage of tweets in each of the six categories in which the tweets are labeled.}
\label{tab:stat}
\end{table}

\section{List of frequent 230 nouns}
The list of 230 nouns that we obtain in the first step of our target word selection scheme can be found in following box.

\fbox{\begin{minipage}{0.43\textwidth}\scriptsize
\textit{`welfare', `anniversary', `tribute', `box', `victory', `thing', `lot', `youth', `need', `nation', `birth', `people', `muslims', `god', `water', `teacher', '`airport', `army', `room', `answer', `blood', `law', `light', `chief', `green', `office', `border', `food', `university', `side', `event', `health', `reason', `city', `station', `theatre', `crore', `ground', `college', `bomb', `corruption', `court', `opposition', `respect', `life', `air', `rail', `student', `government', `mom', `aunty', `weekend', `age', `protest', `guy', `company', `bollywood', `place', `message', `friend', `mind', `mobile', `view', `volunteer', `moment', `rest', `suicide', `lyrics', `group', `death', `home', `way', `brother', `house', `blue', `wedding', `reaction', `terrorist', `person', `mother', `press', `election', `power', `question', `lord', `birthday', `president', `half', `day', `internet', `number', `service', `morning', `waste', `voice', `evening', `night', `luck', `son', `favourite', `captain', `video', `sun', `body', `experience', `family', `use', `music', `date', `teaser', `share', `man', `paper', `lunch', `logo', `season', `job', `game', `post', `gift', `poster', `film', `test', `performance', `price', `plan', `class', `shot', `report', `prime', `state', `exam', `success', `road', `form', `problem', `check', `wife', `boy', `car', `heart', `scam', `style', `police', 'issue', 'card', 'country', 'boss', 'party', 'entry', 'uncle', 'politics', `father', `parliament', `work', `sunday', `story', `play', `request', `week', `playlist', `matter', `superstar', `traffic', `suit', `woman', `cool', `history', `money', `bat', `seat', `score', `photo', `parents', `decision', `girlfriend', `picture', `month', `song', `word', `school', `hero', `degree', `love', `train', `end', `wrong', `main', `scene', `bank', `miss', `king', `channel', `face', `link', `news', `media', `mood', `book', `selfie', `bus', `status', `petrol', `railway', `budget', `well', `development', `team', `phone', `baby', `sir', `interview', `fan', `trailer', `year', `girl', `time', `review', `madam', `movie', `minister', `joke', `century', `cup', `match', `world', `temple', `wicket', `cricket', `star'}
\end{minipage}}

\section{Grouping fot target word selection}
In order to select set of \TG{s} we constructed a feature vector for each of the 230 nouns followed by a K-means clustering. The procedure is as follows.

\noindent{\em Construction of feature vectors} -- We represent a context feature for a \TG~as a tuple $\{P_b, P_a\}$ where $P_b$ is the language tag for the word before the \TG~(i.e., the left context) and $P_a$ is the language tag of the word after the \TG~(i.e., the right context). Each of $P_b$ and $P_a$ can be either ``E'' indicating English, ``H'' indicating Hindi or ``\$'' indicating the boundary (i.e., beginning or end) of the tweet. Thus, we have \textit{eight} feature combinations of the left and the right contexts of a \TG~-- ``EE'', ``HH'', ``EH'', ``HE'', ``\$E'', ``E\$'', ``\$H'', ``H\$'' while ``\$\$'' is not possible. For every \TG, we compute the percentage of occurrences of each of these combinations.   

Note that we compute these percentages from the three different categories of tweets -- \textit{CME}, \textit{CMH} and \textit{CMEQ}. Thus, for every \TG~we have a final feature vector of length 24, each entry denoting the percentage of one feature combination in a particular tweet category. We show example feature vectors for some words in figure~\ref{fig:24Feature}.

\noindent{\em $K$-means clustering} -- We use the feature representation of the words to cluster them into contextually similar groups. We use $K$-means clustering~\cite{hartigan1979algorithm} for this purpose. We vary the value of $K$ and using the traditional elbow method~\cite{tibshirani2001estimating} we obtain 15 as the optimal value of $K$. This process therefore groups the 230 nouns into 15 different clusters. 

\begin{figure}

\centering
\vspace{-3mm}
\caption{Stacked plot representing feature vectors of four different words. Note that the feature vectors of the word pairs (i) ``job'' and ``film'' and (ii) ``moment'' and ``protest'' are very similar. The fractional counts of the eight combinations for each tweet category should sum up to one; since there are three tweet categories so the total size of the stacked plot is three.}
\includegraphics[width=0.49\textwidth]{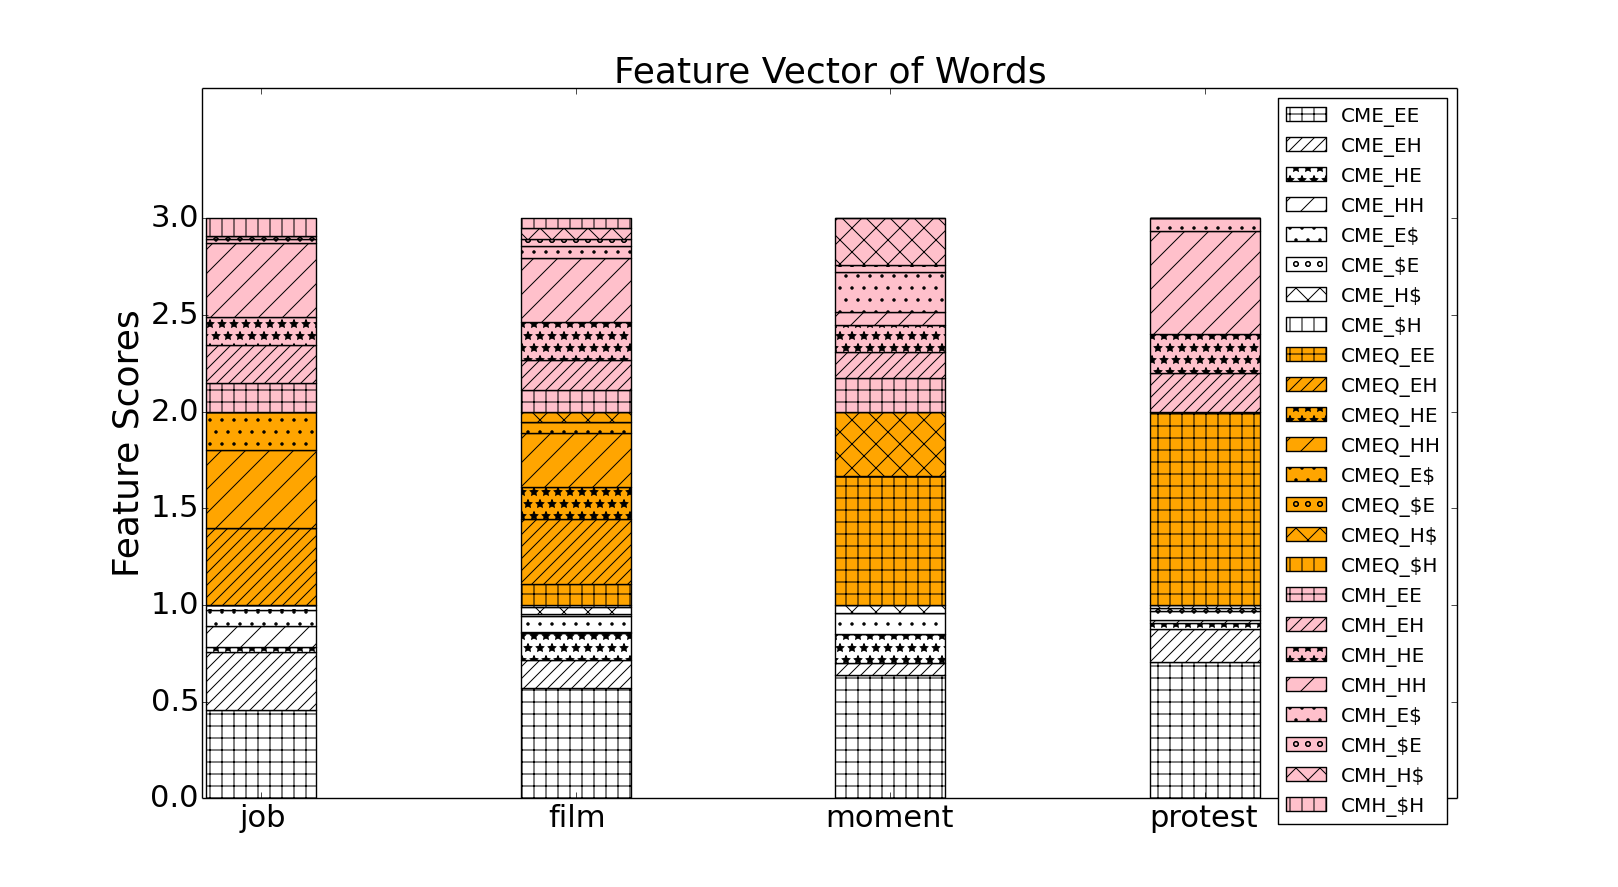}
\label{fig:24Feature}
\vspace{-4mm}
\end{figure}

\section{Age-wise distribution of survey participants}
The age wise distribution of survey participants are presented in figure~\ref{fig:AgeDistribution}. It was on this basis of this distribution that the participants were classified into two classes (young and old).

\begin{figure}
\caption{Age distribution of the survey participants.}
\centering
\vspace{-3mm}
\includegraphics[width=0.5\textwidth]{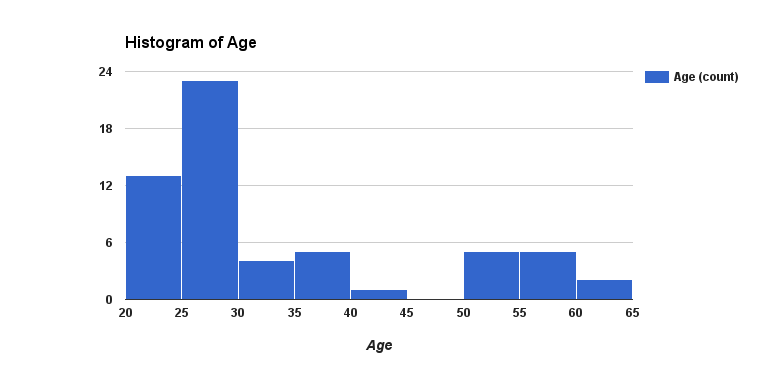}
\label{fig:AgeDistribution}
\end{figure}

\section{Ranked order histograms of \TG{s}}
The ranked order histograms of 57 candidate words according to $LPF$, $UUR$ and the baseline metric are given in Figure~\ref{fig:All_List}.

\begin{figure}
\caption{The rank ordered histograms of \TG\textit{s} ranked by various metrics.}
\centering
\vspace{-3mm}
\includegraphics[width=0.5\textwidth]{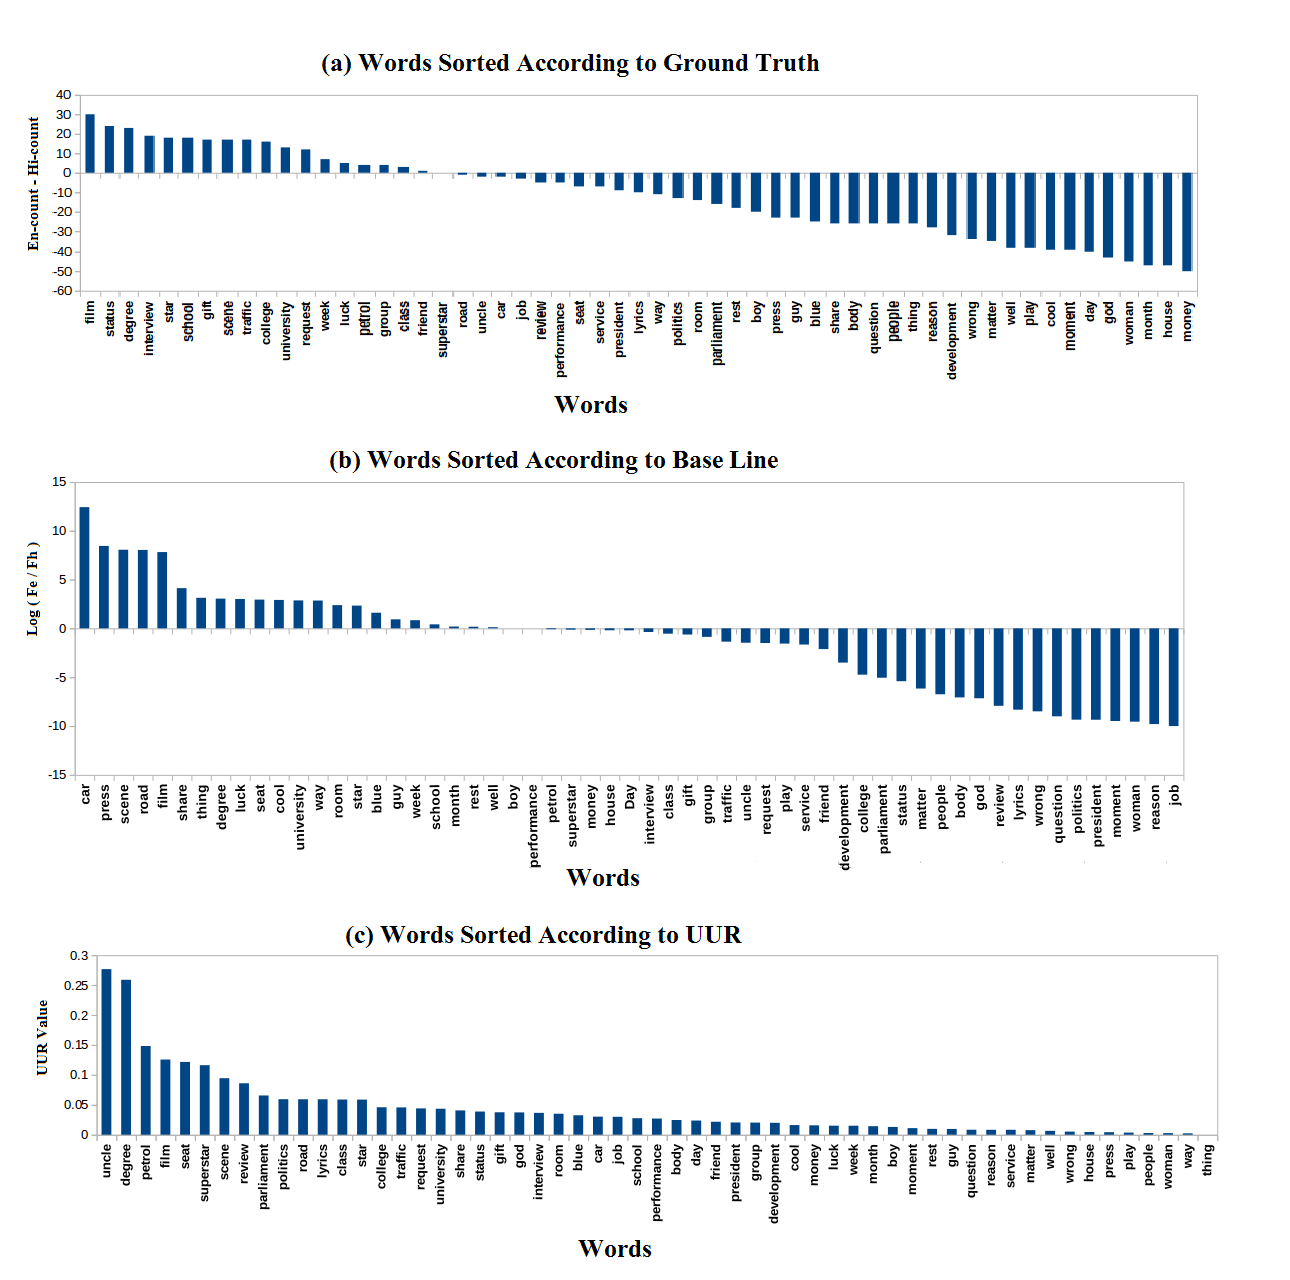}
\label{fig:All_List}
\end{figure}

\end{appendix}
